# Supplementary material for: Social-Group-Agnostic Word Embedding Debiasing via the Stereotype Content Model
Source: arXiv:2210.05831 source file (2022-10-11)
Supplement: Supplementary file 1 [file 6-appendix.tex]

\section{Implementation Details}\label{sec:SM}

\subsection{Training Word Embeddings}
We used Gensim \cite{rehurek2011gensim} implementation of Skip Gram with Negative Sampling variant of Word2Vec \cite{mikolov2013distributed} to train a 300 dimensional word embedding model on the WikiText-103 \cite{merity2016pointer} with a 5-word window. Words with fewer than 5 occurances in the corpus were dropped. Training was done for 5 iterations with 48 threads on a single AMD Ryzen Threadripper 2990WX CPU.

% \section{Details of Debiasing Algorithms and Measurement}

\subsection{Debiasing Algorithms} Algorithms We used \citet{bolukbasi2016man}'s gender word sets and implementation of for HD. For Sub, LP and PP we follow \citet{dev2019attenuating}. The implementation can be found in the project repository. 

\subsection{Bias Subspace} The bias subspace used in HD is identical to that of \citet{bolukbasi2016man}. Each dimensions' bias subspace for Sub, LP, and PP  was the first principal component of C constructed using 8 randomly sampled word pairs from the corresponding dimensions' word pair list (Section~\ref{sec:wordlists}).

\subsection{Experiments}
Each debiasing algorithm for each dimension was conducted 30 times using a random sample of 8 pairs from the corresponding word list. 

\subsection{Word Pairs}
\label{sec:wordlists}

\subsubsection{Social Group Word Pairs}

\smallskip\noindent\textbf{Gender~~} (``nephews'', ``nieces''), (``nephew'', ``niece''),
 (``males'', ``females''),
 (``boys'', ``girls''),
 (``man'', ``woman''),
 (``sons'', ``daughters''),
 (``brother'', ``sister''),
 (``boy'', ``girl''),
 (``father'', ``mother''),
 (``guy'', ``gal''),
 (``male'', ``female''),
 (``uncle'', ``aunt''),
 (``himself'', ``herself''),
 (``uncles'', ``aunts''),
 (``fathers'', ``mothers''),
 (``his'', ``her''),
 (``son'', ``daughter''),
 (``him'', ``her''),
 (``men'', ``women''),
 (``his'', ``hers''),
 (``he'', ``she''),
 (``brothers'', ``sisters''), from \citet{bolukbasi2016man}.
 
\smallskip\noindent\textbf{Race~~} (``Brad'',``Darnell''),
(``Brendan'',``Hakim''),
(``Geoffrey'',``Jermaine''),
(``Greg'',``Kareem''),
(``Brett'',``Jamal''),
(``Neil'',``Rasheed''),
(``Neil'',``Rasheed''),
(``Todd'',``Tyrone''),
(``Allison'',``Aisha''),
(``Anne'',``Ebony''),
(``Carrie'',``Keisha''),
(``Emily'',``Kenya''),
(``Laurie'',``Latoya''),
(``Meredith'',``Tamika''), from \citet{caliskan2017semantics}.

\smallskip\noindent\textbf{Age~~} (``Tiffany'',``Ethel''),
(``Michelle'',``Bernice''),
(``Cindy'',``Gertrude''),
(``Kristy'',``Agnes''),
(``Brad'',``Cecil''),
(``Eric'',``Wilbert''),
(``Joey'',``Mortimer''),
(``Billy'',``Edgar''), from \citet{caliskan2017semantics}.

\subsubsection{SCM Word Pairs}

\smallskip\noindent\textbf{Warmth~~}   (``pleasant'',``unpleasant''),
  (``liked'',``disliked''),
  (``outgoing'',``shy''),
  (``sensitive'',``insensitive''),
  (``friendliness'',``unfriendliness''),
 (``sociable'', ``unsociable''),
 (``warm'', "cold''),
  (``warmth'', "coldness''),
  (``honest'',``dishonest''),
  (``fair'',``unfair''),
  (``loyal'',``disloyal''),
  (``right'',``wrong''),
  (``criminal'',``innocent''),
  (``genuine'',``fake''),
  (``reliable'',``unreliable''), from \citet{nicolas2021comprehensive}.

\smallskip\noindent\textbf{Competence~~}
  (``smart'', ``stupid''),
(``competent'',``incompetent''),
(``intelligent'',``dumb''),
  (``able'', "unable''),
(``rational'',``irrational''),
(``capable'',``incapable''),
  (``aggressive'', "docile''),
(``resilient'',``nonresilient''),
(``motivated'',``unmotivated''),
  (``ambitious'',``unambitious''),
(``independent'',``dependent''),
(``determined'',``inactive''),
  (``secure'',``insecure''),
(``clever'',``foolish''),
(``dominant'',``submissive''), from \citet{nicolas2021comprehensive}.

% \section{Experiment Details}

% \begin{itemize}
%     \item Corpus for word embeddings
%     \item Word embedding algorithm and training parameters
%     \item Selection of any parameters or decisions for baseline algorithms (HD, etc.)
%     \item List all word lists used (done)
%     \item Discuss repetition of debiasing and the number of repetitions
% \end{itemize}

%\section{Additional Results}

% Once the SCM bias subspace is determined, we follow the procedure of \cite{dev2019attenuating} to remove bias via partial projection (see section \ref{sec:debias_algos})  using $f_1$ and $\sigma=1$. For NBM, we set $k=100$ and for all bias measures, the final bias score of a word $w$ is the average score across all word pairs of a protected attribute.
